# Supplementary material for: Z-STAR+: A Zero-shot Style Transfer Method via Adjusting Style Distribution
Source: arXiv:2411.19231 source file (2024-11-28)
Supplement: Supplementary file 3 [file fig_supp_big.tex]

\newcommand\bigfigurewidth{0.31}

\begin{figure*}%[t]
\centering
\includegraphics[width=\bigfigurewidth\linewidth]{image/figs_bigs/c1.png}
\includegraphics[width=\bigfigurewidth\linewidth]{image/figs_bigs/r1.png}
\includegraphics[width=\bigfigurewidth\linewidth,height=\bigfigurewidth\linewidth]{image/figs_bigs/s1.png}

\includegraphics[width=\bigfigurewidth\linewidth]{image/figs_bigs/c2.png}
\includegraphics[width=\bigfigurewidth\linewidth]{image/figs_bigs/r2.png}
\includegraphics[width=\bigfigurewidth\linewidth,height=\bigfigurewidth\linewidth]{image/figs_bigs/s2.png}

\includegraphics[width=\bigfigurewidth\linewidth]{image/figs_bigs/c3.png}
\includegraphics[width=\bigfigurewidth\linewidth]{image/figs_bigs/r3.png}
\includegraphics[width=\bigfigurewidth\linewidth,height=\bigfigurewidth\linewidth]{image/figs_bigs/s3.png}

\includegraphics[width=\bigfigurewidth\linewidth]{image/figs_bigs/c4.png}
\includegraphics[width=\bigfigurewidth\linewidth]{image/figs_bigs/r4.png}
\includegraphics[width=\bigfigurewidth\linewidth,height=\bigfigurewidth\linewidth]{image/figs_bigs/s4.png}

\vspace{-2pt}
\begin{minipage}{\bigfigurewidth\linewidth}
    \centering
    \figtext{Content}
\end{minipage}
\begin{minipage}{\bigfigurewidth\linewidth}
    \centering
    \figtext{Our results}
\end{minipage}
\begin{minipage}{\bigfigurewidth\linewidth}
    \centering
    \figtext{Style}
\end{minipage}
\vspace{-7pt}
\caption{More style transfer results in a large resolution of $768 \times 768$.
% The first column shows content images, the second column shows style images. The remaining columns are stylized results generated by different methods.
}\label{fig:big}
\end{figure*}
